# Supplementary material for: Surface response of a polymer network: Semi-infinite network
Source: arXiv:2003.09048 ancillary file (2020-03-19)

# Surface response of a polymer network: Semi-infinite network

## Supplemental Material

This file is a supplement to the article entitled "Surface response of a polymer network: Semi-infinite network", by Chen Bar-Haim and Haim Diamant, submitted to Langmuir.
It gives the detailed calculations leading to the results presented in the article.
The work is based on the two-fluid model. We calculate: (i) the decay rate (dispersion relation) of surface fluctuations as a function of wavevector; (ii) the displacement and velocity response to a localized force applied to the surface.
The surface lies on the plane (x, y, z = 0) and the material occupies the half-space z < 0. We use a 2D Fourier transform for (x,y) → (qx,qy) and leave z in real space.
For the rest of the symbols see the main text.

# Definitions

```
In[ ]:= grad[f_] := {ⅈ qx f, ⅈ qy f, ∂z f} (* gradient of scalar function f *)

In[ ]:= div[v_] := ⅈ qx v[[1]] + ⅈ qy v[[2]] + ∂z v[[3]] (* divergence of vector function v *)

In[ ]:= lap[f_] := -qx^2 f - qy^2 f + ∂z,z f (* Laplacian of scalar function f *)

In[ ]:= veclap[v_] := -qx^2 v - qy^2 v + ∂z,z v (* Laplacian of vector function v *)

In[ ]:= curl[v_] := {ⅈ qy v[[3]] - ∂z v[[2]], ∂z v[[1]] - ⅈ qx v[[3]], ⅈ qx v[[2]] - ⅈ qy v[[1]]}
          (* curl of vector function v *)
```

# Model equations

There are 7 equations total: two 3-vector equations + one scalar equation, for the two 3-vector fields (v, u) and one scalar field (p).
The following 3 expressions should vanish.

```
In[ ]:= eq01 := -grad[p[qx, qy, z]] + η veclap[v[qx, qy, z]] -
           Γ (v[qx, qy, z] - ⅈ ω u[qx, qy, z]) + 0 * fv[qx, qy, z];
        (* Stokes + mutual friction for the fluid *)
```

```
In[ ]:= eq02 := G (veclap[u[qx, qy, z]]) + (K + G / 3) grad[div[u[qx, qy, z]]] -
           Γ (ⅈ ω u[qx, qy, z] - v[qx, qy, z]) + 0 * fu[qx, qy, z];
        (* Elasticity + mutual friction for the network *)
```

```
In[ ]:= eq03 := div[v[qx, qy, z]];
        (* Fluid incompressibility, approximately equal to medium incompressibility *)
```

```
In[ ]:= eq04 := -ⅈ ω Γ div[u[qx, qy, z]] + lap[p[qx, qy, z]] - 0 * div[fv[qx, qy, z]];
        (* An auxilary equation obtained from the div of eq01 *)
```

## Switching parameters

from (G, Γ, K) to ($\eta$b, $\xi$, $\lambda$)

```
In[ ]:= G = ⅈ ω (ηb - η); (* introducing bulk viscosity ηb=η+G/ⅈω *)
        Γ = η G / (ⅈ ω ηb ξ^2); (* introducing transverse length ξ *)
        K = (λ^2 ⅈ ω Γ) - 4 G / 3; (* introducing longitudinal length λ;
        λ^2/ξ^2 = (ηb/η) 2(1-ν)/(1-2ν); λ diverges for an incompressible network *)
```

# Decoupled equations

Define two flows, Vc,Vr, which are combinations of v and u such that the equations decouple. (See ref 18 in the paper.)

Vc is the collective flow of the two fluids; Vr is the relative flow.

Add to each of them a term proportional to grad[p] to make both flows incompressible.

Vc turns out to satisfy the Stokes equation. Vr turns out to satisfy the Brinkman equation.

Vc = (1 - $\eta$/$\eta$b) ($i\omega$u + ($\eta$/($\eta$b-$\eta$)) v - 1/Γ grad[p])

Vr = ($\eta$b/$\eta$ - 1) ($i\omega$u - v - 1/Γ grad[p])

P = p - $\lambda^2$ lap[p]

```
In[ ]:= Vc[x_, y_, z_] = {Vcx[qx, qy, z], Vcy[qx, qy, z], Vcz[qx, qy, z]};
        Vr[x_, y_, z_] = {Vrx[qx, qy, z], Vry[qx, qy, z], Vrz[qx, qy, z]};
```

eq01,...,eq04 turn into the following 4 expressions which should vanish.

```
In[ ]:= eq11 = -grad[P[qx, qy, z]] + (η + G / (ⅈ ω)) veclap[Vc[qx, qy, z]];
```

```
In[ ]:= eq12 =
          -grad[P[qx, qy, z]] + η veclap[Vr[qx, qy, z]] - (ⅈ ω Γ (G + ⅈ ω η) / G) Vr[qx, qy, z];
```

```
In[ ]:= eq13 = div[Vc[qx, qy, z]];
```

```
In[ ]:= eq14 = div[Vr[qx, qy, z]];
```

# Solve for the collective flow $V_c$

## Equations for $V_c$

Vc satisfies the Stokes equation of an incompressible fluid.

In[ ]:=
```
eq21 = -ⅈ qx P[qx, qy, z] + ηb ((-qx^2 - qy^2) Vcx[qx, qy, z] + Vcx^(0,0,2)[qx, qy, z]);
eq22 = -ⅈ qy P[qx, qy, z] + ηb ((-qx^2 - qy^2) Vcy[qx, qy, z] + Vcy^(0,0,2)[qx, qy, z]);
eq23 = -P^(0,0,1)[qx, qy, z] + ηb ((-qx^2 - qy^2) Vcz[qx, qy, z] + Vcz^(0,0,2)[qx, qy, z]);
eq24 = ⅈ qx Vcx[qx, qy, z] + ⅈ qy Vcy[qx, qy, z] + Vcz^(0,0,1)[qx, qy, z];
```

## Solution for $V_c$

The following expressions give the solution of eq21-eq24 for Vc. Terms which diverge at z → -∞ have been removed.
We check this solution below.

In[ ]:= $A = \sqrt{qx^2 + qy^2}$;

In[ ]:= Vcx[qx_, qy_, z_] = $C6\, e^{-A z} - \frac{i\, C4\, e^{-A z}\, qx\, z}{A}$;

In[ ]:= Vcy[qx_, qy_, z_] = $C8\, e^{-A z} - \frac{i\, C4\, e^{-A z}\, qy\, z}{A}$;

In[ ]:= Vcz[qx_, qy_, z_] = $C3\, e^{-A z} + C4\, e^{-A z}\, z$;

# Solve for the relative flow $V_r$

## Equations for $V_r$

Vr satisfies the Brinkman equation of an incompressible fluid.

```
In[•]:= eq31 = - ⅈ qx P[qx, qy, z] +
            η ((-qx^2 - qy^2) Vrx[qx, qy, z] + Vrx^(0,0,2)[qx, qy, z] - ξ^-2 Vrx[qx, qy, z]);
        eq32 = - ⅈ qy P[qx, qy, z] +
            η ((-qx^2 - qy^2) Vry[qx, qy, z] + Vry^(0,0,2)[qx, qy, z] - ξ^-2 Vry[qx, qy, z]);
        eq33 = - P^(0,0,1)[qx, qy, z] +
            η ((-qx^2 - qy^2) Vrz[qx, qy, z] + Vrz^(0,0,2)[qx, qy, z] - ξ^-2 Vrz[qx, qy, z]);
        eq34 = ⅈ qx Vrx[qx, qy, z] + ⅈ qy Vry[qx, qy, z] + Vrz^(0,0,1)[qx, qy, z];
```

## Solution for $V_r$

The following expressions give the solution of eq31-eq34 for Vc. Terms which diverge at z → -∞ have been removed.

We check this solution below.

```
In[•]:= B = Sqrt[1 + qx^2 ξ^2 + qy^2 ξ^2] / ξ;

In[•]:= Vrx[qx_, qy_, z_] = D6 e^(-B z) - (ⅈ D2 e^(-A z) qx) / A;

In[•]:= Vry[qx_, qy_, z_] = D8 e^(-B z) - (ⅈ D2 e^(-A z) qy) / A;

In[•]:= Vrz[qx_, qy_, z_] = D2 * Exp[-A * z] + D4 * Exp[-B * z];
```

# Solve for the pressure P

```
In[•]:= P[qx_, qy_, z_] = 2 C4 e^(-A z) ηb;
```

P for both sets of equations must be the same. This eliminates one integration constant.

```
In[•]:= s1 = Solve[2 ηb C4 == η D2 / (A ξ^2), D2];

In[•]:= D2 = D2 /. s1[[1]];
```

# Check solution for decoupled equations

## Check the solution for $V_c$

We use the incompressibility equation to eliminate another integration constant.

```
In[•]:= s2 = Solve[I * qx * Vcx[qx, qy, z] + I * qy * Vcy[qx, qy, z] + D[Vcz[qx, qy, z], z] == 0 , C3];
```

In[ ]:=
```
C3 = C3 /. s2[[1]];
```

Check validity of Vc solution.

In[ ]:=
```
FullSimplify[{eq21, eq22, eq23, eq24}, ξ > 0]
```

Out[ ]=
```
{0, 0, 0, 0}
```

## Check the solution for $V_r$

We use the incompressibility equation to eliminate another integration constant.

In[ ]:=
```
s3 = Solve[I * qx * Vrx[qx, qy, z] + I * qy * Vry[qx, qy, z] + D[Vrz[qx, qy, z], z] == 0 , D4];
```

In[ ]:=
```
D4 = D4 /. s3[[1]];
```

Check validity of Vr solution.

In[ ]:=
```
FullSimplify[{eq31, eq32, eq33, eq34}, ξ > 0]
```

Out[ ]=
```
{0, 0, 0, 0}
```

# Check solution for original, coupled equations

## Finding original flows

Vc = (1 - η/ηb) (ⅈωu + (η/(ηb-η)) v - 1/Γ grad[p])
Vr = (ηb/η - 1) (ⅈωu - v - 1/Γ grad[p])
P = p - $\lambda^2$ lap[p]

In[ ]:=
```
FullSimplify[p[qx, qy, z] - λ^2 * lap[p[qx, qy, z]]] - P[qx, qy, z]
```

Out[ ]=
$$-2\,C4\,e^{-\sqrt{qx^2+qy^2}\,z}\,\eta b + \left(1 + \left(qx^2 + qy^2\right)\lambda^2\right) p[qx, qy, z] - \lambda^2\, p^{(0,0,2)}[qx, qy, z]$$

In[ ]:=
$$p[qx\_, qy\_, z\_] = e^{-H z}\,E2 + 2\,C4\,e^{-A z}\,\eta b;$$

In[ ]:=
$$v[qx\_, qy\_, z\_] = -\frac{Vr[qx, qy, z]\,\eta - Vc[qx, qy, z]\,\eta b}{\eta b};$$

In[ ]:=
$$u[qx\_, qy\_, z\_] = \frac{1}{\eta\,(\eta - \eta b)\,\eta b\,\omega}\, i\left(\eta b^2\,\xi^2\,grad[p[qx, qy, z]] + \eta\,\eta b\,(-\eta + \eta b)\,Vc[qx, qy, z] + \eta^3\,Vr[qx, qy, z]\right);$$

In[ ]:= $H = \frac{\sqrt{1 + qx^2 \lambda^2 + qy^2 \lambda^2}}{\lambda}$;

## Check that the original equations are satisfied

```
In[ ]:= FullSimplify[{eq01, eq02, eq03, eq04}]
Out[ ]= {{0, 0, 0}, {0, 0, 0}, 0, 0}
```

# Expressions for stress tensors

```
In[ ]:= {vx[qx_, qy_, z_], vy[qx_, qy_, z_], vz[qx_, qy_, z_]} = v[qx, qy, z];
In[ ]:= {ux[qx_, qy_, z_], uy[qx_, qy_, z_], uz[qx_, qy_, z_]} = u[qx, qy, z];
```

## Stress tensor of the viscous fluid

```
In[ ]:= σvxz = FullSimplify[η (D[vx[qx, qy, z], z] + I qx vz[qx, qy, z])];
In[ ]:= σvyz = FullSimplify[η (D[vy[qx, qy, z], z] + I qy vz[qx, qy, z])];
In[ ]:= σvzz = FullSimplify[2 η D[vz[qx, qy, z], z] - p[qx, qy, z]];
```

## Stress tensor of the (visco)elastic network

```
In[ ]:= σuxz = FullSimplify[G (D[ux[qx, qy, z], z] + I qx uz[qx, qy, z]) /. {G → (ηb - η) I ω}];
In[ ]:= σuyz = FullSimplify[G (D[uy[qx, qy, z], z] + I qy uz[qx, qy, z]) /. {G → (ηb - η) I ω}];
In[ ]:= σuzz = Simplify[2 G D[uz[qx, qy, z], z] +
          (K - 2 G / 3) (I qx ux[qx, qy, z] + I qy uy[qx, qy, z] + D[uz[qx, qy, z], z])];
```

# Calculate dispersion relation ω(qx,qy)

We apply the same boundary conditions but without external force.

```
In[ ]:= eqn1 = σvxz + σuxz == 0;
In[ ]:= eqn2 = σvyz + σuyz == 0;
In[ ]:= eqn3 = σvzz + σuzz + γ (qx^2 + qy^2) uz[qx, qy, z] == 0;
In[ ]:= eqn4 = I * ω * ux[qx, qy, z] - vx[qx, qy, z] == 0;
In[ ]:= eqn5 = I * ω * uy[qx, qy, z] - vy[qx, qy, z] == 0;
```

In[ ]:=
```
eqn6 = I * ω * uz[qx, qy, z] - vz[qx, qy, z] == 0;
```

Set z to zero (calculate on surface)

In[ ]:=
```
eqn1 = eqn1 //. z → 0; eqn2 = eqn2 //. z → 0; eqn3 = eqn3 //. z → 0;
eqn4 = eqn4 //. z → 0; eqn5 = eqn5 //. z → 0; eqn6 = eqn6 //. z → 0;
```

Construct the matrix of coefficients

In[ ]:=
```
CoefficientArrays[{eqn1, eqn2, eqn3, eqn4, eqn5, eqn6}, {C6, C4, D6, C8, D8, E2}];
```

In[ ]:=
```
(Normal[%][[2]]) // MatrixForm
```

Out[ ]//MatrixForm=

$$\begin{pmatrix}
-\frac{\left(2\,qx^2+qy^2\right)\,\eta}{\sqrt{qx^2+qy^2}}-\frac{\left(2\,qx^2+qy^2\right)\,(-\eta+\eta b)}{\sqrt{qx^2+qy^2}} & -4\,i\,qx\,\sqrt{qx^2+qy^2}\,\eta\,\xi^2-\frac{4\,i\,qx\,\sqrt{q\ldots}}{\ldots} \\
-\frac{qx\,qy\,\eta}{\sqrt{qx^2+qy^2}}-\frac{qx\,qy\,(-\eta+\eta b)}{\sqrt{qx^2+qy^2}} & -4\,i\,qy\,\sqrt{qx^2+qy^2}\,\eta\,\xi^2-\frac{4\,i\,qy\,\sqrt{q\ldots}}{\ldots} \\
-2\,i\,qx\,\eta+2\,i\,qx\,(\eta-\eta b)-\frac{qx\,\sqrt{qx^2+qy^2}\,\gamma\,(-\eta+\eta b)}{(\eta-\eta b)\,\omega} & -2\,\eta b+4\left(qx^2+qy^2\right)\eta\,\xi^2-\frac{4\left(qx^2+qy^2\right)(\eta-\eta b)\,(\eta+\eta b)\,\xi^2}{\eta} \\
-1-\frac{-\eta+\eta b}{\eta-\eta b} & -2\,i\,qx\,\xi^2+\ldots \\
0 & -2\,i\,qy\,\xi^2+\ldots \\
-\frac{i\,qx}{\sqrt{qx^2+qy^2}}-\frac{i\,qx\,(-\eta+\eta b)}{\sqrt{qx^2+qy^2}\,(\eta-\eta b)} & -\frac{1}{\sqrt{qx^2+qy^2}}-\frac{-\eta+\eta b}{\sqrt{qx^2+qy^2}\,(\eta-\eta b)}+2\,\sqrt{q\ldots}
\end{pmatrix}$$

Setting the determinant to zero gives the equation for $\omega$

In[ ]:=
```
s2 = Solve[Det[%] == 0, ω];
```

In[ ]:=
```
ωDR = ω /. s2[[1]];
```

In[ ]:=
```
ωDR = FullSimplify[
   ωDR /. {B → Sqrt[1 + qx^2 ξ^2 + qy^2 ξ^2]/ξ, A → Sqrt[qx^2 + qy^2], H → Sqrt[1 + qx^2 λ^2 + qy^2 λ^2]/λ}];
(* to simplfy the expression *)
```

In[ ]:=
```
ωDR = FullSimplify[% /. {Sqrt[qx^2 + qy^2] → q, (qx^2 + qy^2) → q^2}]
```

Out[ ]=

$$\left(i\,q\,\gamma\,\eta\left(\sqrt{1+q^2\lambda^2}+q^2\,\xi\left(\sqrt{1+q^2\lambda^2}\;\xi-\lambda\sqrt{1+q^2\xi^2}\right)\right)\right)\Big/\left(2\,\eta b\left(2\,q^2\,\eta b\left(-q\,\lambda+\sqrt{1+q^2\lambda^2}\right)\xi^2\left(1+q\,\xi\left(q\,\xi-\sqrt{1+q^2\xi^2}\right)\right)+\eta\left(-\sqrt{1+q^2\lambda^2}+q^2\,\xi\left(-3\sqrt{1+q^2\lambda^2}\;\xi+2\,q^3\,\lambda\,\xi^3+\lambda\sqrt{1+q^2\xi^2}-2\,q^2\,\xi^2\left(\sqrt{1+q^2\lambda^2}\;\xi+\lambda\sqrt{1+q^2\xi^2}\right)+2\,q\,\xi\left(\lambda+\sqrt{1+q^2\lambda^2}\;\xi\sqrt{1+q^2\xi^2}\right)\right)\right)\right)\right)$$

# Check asymptotic behavior of $\omega$

## Small q

In[ ]:=
```
Series[ωDR, {q, 0, 1}]
```

Out[ ]=

$$-\frac{i\,\gamma\,q}{2\,\eta b}+O[q]^2$$

$$-i\,\omega = \frac{\gamma\,q}{2\,\eta_b} \quad \text{for } q << \lambda^{-1}$$

## Large q

The large-q limit is harder to find. We expand instead in large $\eta$b, which means large $\lambda$ (i.e., small 1/$\lambda$ relative to q).

We (a) normalize the parameters; (b) expand the numerator and denominator in large $\eta$b; (c) regroup; (d) remove normalization.

In[ ]:=
```
DRLargeq = FullSimplify[-I * ωDR /. {ξ → 1, η → 1, γ → 1}];
```

In[ ]:=
```
DRLargeq = FullSimplify[% /. {λ → Sqrt[ηb] * β}, ηb > 0]
```

Out[ ]=

$$-\left(\left(q\left(\sqrt{1+q^2\beta^2\eta b}+q^2\left(-\beta\sqrt{(1+q^2)\,\eta b}+\sqrt{1+q^2\beta^2\eta b}\right)\right)\right)\Big/\left(2\,\eta b\left(\sqrt{1+q^2\beta^2\eta b}+q^2\left(2\,q^3\beta\,(-1+\eta b)\sqrt{\eta b}-\beta\sqrt{(1+q^2)\,\eta b}+(3-2\,\eta b)\sqrt{1+q^2\beta^2\eta b}-2\,q^2\,(-1+\eta b)\left(\beta\sqrt{(1+q^2)\,\eta b}+\sqrt{1+q^2\beta^2\eta b}\right)+2\,q\,(-1+\eta b)\left(\beta\sqrt{\eta b}+\sqrt{1+q^2}\sqrt{1+q^2\beta^2\eta b}\right)\right)\right)\right)\right)$$

In[ ]:= 
```
FullSimplify[Denominator[DRLargeq] /. ηb → x^2, {x > 0, β > 0, q > 0}]
```

Out[ ]= 
$$2x^2\left(\sqrt{1+q^2x^2\beta^2}+q^2\left(-\sqrt{1+q^2}\,x\beta+2q^3x\left(-1+x^2\right)\beta+\left(3-2x^2\right)\sqrt{1+q^2x^2\beta^2}-2q^2\left(-1+x^2\right)\left(\sqrt{1+q^2}\,x\beta+\sqrt{1+q^2x^2\beta^2}\right)+2q\left(-1+x^2\right)\left(x\beta+\sqrt{\left(1+q^2\right)\left(1+q^2x^2\beta^2\right)}\right)\right)\right)$$

In[ ]:= 
```
FullSimplify[Series[%, {x, Infinity, 1}], {x > 0, β > 0, q > 0}]
```

Out[ ]= 
$$\frac{2q\left(1+q^2-q\sqrt{1+q^2}\right)\left(-1+\beta^2\right)x^3}{\beta}+\frac{\left(1+2\beta^2+q\left(q-\sqrt{1+q^2}+q\left(6+4q\left(q-\sqrt{1+q^2}\right)\right)\beta^2\right)\right)x}{2q\beta^3}+O\left[\frac{1}{x}\right]^2$$

In[ ]:= 
```
FullSimplify[Numerator[DRLargeq] /. ηb → x^2, {x > 0, β > 0, q > 0}]
```

Out[ ]= 
$$-q\left(\sqrt{1+q^2x^2\beta^2}+q^2\left(-\sqrt{1+q^2}\,x\beta+\sqrt{1+q^2x^2\beta^2}\right)\right)$$

In[ ]:= 
```
FullSimplify[Series[%, {x, Infinity, 2}], {x > 0, β > 0, q > 0}]
```

Out[ ]= 
$$-q^2\left(1+q^2-q\sqrt{1+q^2}\right)\beta x-\frac{1+q^2}{2\beta x}+O\left[\frac{1}{x}\right]^3$$

In[ ]:= 
$$\text{FullSimplify}\left[-\beta q^2\left(1+q^2-q\sqrt{1+q^2}\right)x\Big/\left(\frac{2\left(-1+\beta^2\right)q\left(1+q^2-q\sqrt{1+q^2}\right)x^3}{\beta}\right)\right]$$

Out[ ]= 
$$-\frac{q\beta^2}{2x^2\left(-1+\beta^2\right)}$$

Going back to the original parameters:

$$-i\omega=\frac{\beta^2 q\gamma}{2\left(\beta^2-1\right)\eta_b}\qquad \text{for } \lambda^{-1} << q << \xi^{-1}$$

# Plot Dispersion relation

In[ ]:= 
```
DRPlot = FullSimplify[-I * ωDR /. {ξ → 1, η → 1, γ → 1, λ → Sqrt[ηb] * β}, ηb > 0];
```

$\beta$ is Sqrt[2 (1 - $\nu$)/(1 - 2$\nu$)]

In[ ]:=
```
LogLogPlot[
 {(-DRPlot) /. {ηb → 100, β → Sqrt[2 (1 - 0.1) / (1 - 2 * 0.1)]}, q/(2 ηb) /. {ηb → 100},
  q/(2 ηb) β^2/(β^2 - 1) /. {ηb → 100, β → Sqrt[2 (1 - 0.1) / (1 - 2 * 0.1)]}}, {q, 0.001, 1},
 PlotRange → All, PlotLegends → {"iω(q)", "q/(2 ηb)", "q/(2 ηb) β²/(β² - 1)"},
 AxesLabel → {"q×ξ", "iω/Ω"}, PlotTheme → "ThickLines"]
```

Out[ ]=

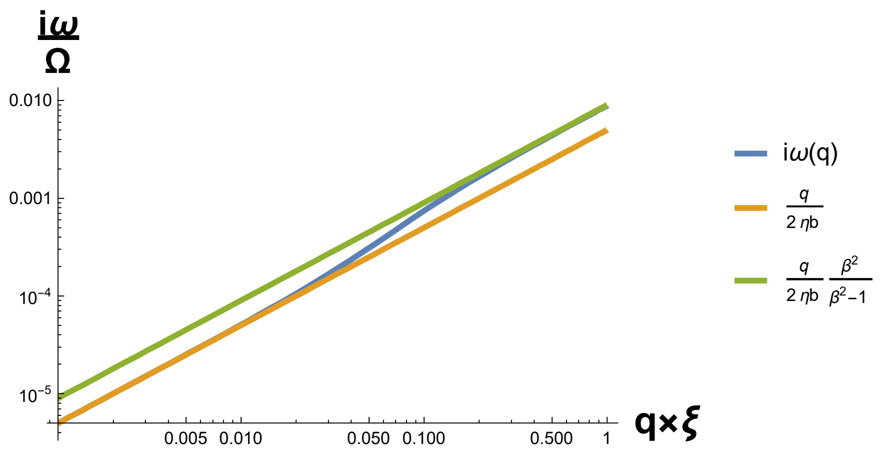


# Surface response

Solve again the boundary condition but this time with force Fx.

In[ ]:=
```
s5 = Solve[{σvxz + σuxz == Fx, σvyz + σuyz == 0, σvzz + σuzz == -γ (q^2) uz[qx, qy, z],
    I * ω * ux[qx, qy, z] == vx[qx, qy, z], I * ω * uy[qx, qy, z] == vy[qx, qy, z],
    I * ω * uz[qx, qy, z] == vz[qx, qy, z]} /. z → 0, {C6, C4, D6, C8, D8, E2}];
```

We extract from the solution the fluid velocities and pressure at the surface.
(The network displacement rate at the surface is equal to the fluid velocity there.)
We apply some manipulations to make the expressions simpler.

In[ ]:=
```
vxSurface = vx[qx, qy, 0] /. s5[[1]];
```

```
In[ ]:= vxSurfaceN = Simplify[vxSurface //. {√(qx² + qy²) → q}];
vxSurfaceN = Simplify[vxSurfaceN //. {qx² ξ² + qy² ξ² → q^2 ξ²}];
vxSurfaceN = Simplify[vxSurfaceN //. {qx² λ² + qy² λ² → q^2 λ²}];
vxSurfaceN = Simplify[vxSurfaceN //. {(qx² + qy²) → q^2}];
vxSurfaceN = Simplify[vxSurfaceN //. {ⅈ qx² γ + ⅈ qy² γ → I q^2 γ}];

In[ ]:= vySurface = vy[qx, qy, 0] /. s5[[1]];

In[ ]:= vySurfaceN = Simplify[vySurface //. {√(qx² + qy²) → q}];
vySurfaceN = Simplify[vySurfaceN //. {qx² ξ² + qy² ξ² → q^2 ξ²}];
vySurfaceN = Simplify[vySurfaceN //. {qx² λ² + qy² λ² → q^2 λ²}];
vySurfaceN = Simplify[vySurfaceN //. {(qx² + qy²) → q^2}];
vySurfaceN = Simplify[vySurfaceN //. {ⅈ qx² γ + ⅈ qy² γ → I q^2 γ}];

In[ ]:= vzSurface = vz[qx, qy, 0] /. s5[[1]];

In[ ]:= vzSurfaceN = Simplify[vzSurface //. {√(qx² + qy²) → q}];
vzSurfaceN = Simplify[vzSurfaceN //. {qx² ξ² + qy² ξ² → q^2 ξ²}];
vzSurfaceN = Simplify[vzSurfaceN //. {qx² λ² + qy² λ² → q^2 λ²}];
vzSurfaceN = Simplify[vzSurfaceN //. {(qx² + qy²) → q^2}];
vzSurfaceN = Simplify[vzSurfaceN //. {ⅈ qx² γ + ⅈ qy² γ → I q^2 γ}];

In[ ]:= pSurface = p[qx, qy, 0] /. s5[[1]];

In[ ]:= pSurfaceN = Simplify[pSurface //. {√(qx² + qy²) → q}];
pSurfaceN = Simplify[pSurfaceN //. {qx² ξ² + qy² ξ² → q^2 ξ²}];
pSurfaceN = Simplify[pSurfaceN //. {qx² λ² + qy² λ² → q^2 λ²}];
pSurfaceN = Simplify[pSurfaceN //. {(qx² + qy²) → q^2}];
pSurfaceN = Simplify[pSurfaceN //. {ⅈ qx² γ + ⅈ qy² γ → I q^2 γ}];
```

# Response functions $G_{xx}$ and $G_{xy}$ in asymptotic limits

Since F is in the x direction, vx gives Gxx and vy gives Gxy

# Small q (large ρ)

In[ ]:=
```
vx0 = vxSurfaceN /. {qx → a * Qx, qy → a * Qy, q → a * Q};
(* a is an expansion parameter *)
```

The expansion contains the leading term and additional spurious ones.

In[ ]:=
```
vx1 = Normal[Series[vx0, {a, 0, 0}]]
```

Out[ ]=
$$-\frac{Fx\sqrt{a^2 Q^2}\,(Qx^2+2\,Qy^2)}{2\,a^2\,Q^4\,\eta b}+\frac{1}{4\,Q^4\,\eta\,\eta b^2\,\omega}\left(-i\,Fx\,Q^2\,Qx^2\,\gamma\,\eta-2\,i\,Fx\,Q^2\,Qy^2\,\gamma\,\eta-4\,Fx\sqrt{a^2 Q^2}\,Qx^4\,\eta b^2\,\xi^2\,\omega-4\,Fx\sqrt{a^2 Q^2}\,Qx^2\,Qy^2\,\eta b^2\,\xi^2\,\omega\right)$$

In[ ]:=
```
vy0 = vySurfaceN /. {qx → a * Qx, qy → a * Qy, q → a * Q};
(* a is an expansion parameter *)
```

The expansion contains the leading term and additional spurious ones.

In[ ]:=
```
vy1 = Normal[Series[vy0, {a, 0, 0}]]
```

Out[ ]=
$$\frac{Fx\sqrt{a^2 Q^2}\,Qx\,Qy}{2\,a^2\,Q^4\,\eta b}-\frac{Fx\sqrt{a^2 Q^2}\,Qx^3\,Qy\,\xi^2}{Q^4\,\eta}-\frac{Fx\sqrt{a^2 Q^2}\,Qx\,Qy^3\,\xi^2}{Q^4\,\eta}+\frac{i\,Fx\,Qx\,Qy\,\gamma}{4\,Q^2\,\eta b^2\,\omega}$$

In[ ]:=
```
vz0 = vzSurfaceN /. {qx → a * Qx, qy → a * Qy, q → a * Q};
(* a is an expansion parameter *)
```

In[ ]:=
```
vz1 = Normal[Series[vz0, {a, 0, 0}]]
```

Out[ ]=
$$-\frac{i\,Fx\sqrt{a^2 Q^2}\,Qx\,(\eta-\eta b)\,\xi^2}{Q\,\eta\,\eta b}$$

In[ ]:=
```
p0 = pSurfaceN /. {qx → a * Qx, qy → a * Qy, q → a * Q}; (* a is an expansion parameter *)
```

In[ ]:=
```
p1 = Normal[Series[p0, {a, 0, 0}]]
```

Out[ ]=
$$\frac{i\,Fx\sqrt{a^2 Q^2}\,Qx}{a\,Q^2}+\frac{i\,Fx\sqrt{a^2 Q^2}\,Qx\,(\eta-\eta b)\,\lambda}{Q\,\eta b}$$

So, in summary, the asymptotic expressions for small q (along with their inversion to real-space q→ρ):

$$Gxx\,(q) = -\frac{qx^2+2\,qy^2}{2\,\eta_b\,q^3} \qquad (q << \lambda)$$

$$\mathrm{Gxx}\ (\rho) = \frac{2\,x^2 + y^2}{4\,\pi\,\eta_b\,\rho^3} \qquad (\rho >> \lambda)$$

$$\mathrm{Gxy}\ (q) = -\frac{qx\,qy}{2\,\eta_b\,q^3} \qquad (q << \lambda)$$

$$\mathrm{Gxy}\ (\rho) = \frac{x\,y}{4\,\pi\,\eta_b\,\rho^3} \qquad (\rho >> \lambda)$$

These bulk results coincide with Landau&Lifshitz Elasticity Sec. 8 (surface response of elastic solid) , once we set there $\nu = 1/2$ and G = i $\omega\,\eta$b.

An example of inversion to real space (of Gxy):

$$\mathrm{Gxy} = \frac{\mathrm{Fx}\sqrt{Q^2}\ \mathrm{Qx\,Qy}}{2\,a\,Q^4\,\eta b}$$

In[ ]:=
```
InverseFourierTransform[1/ (qx^2 + qy^2)^(3/2) , {qx, qy}, {x, y}]
```

Out[ ]= $-\sqrt{x^2 + y^2}$

In[ ]:=
```
GxxRealSpace1 = FullSimplify[(D[D[-Sqrt[x^2 + y^2] , x], y])/ (2 ηb)]
```

Out[ ]= $$\frac{x\,y}{2\,\left(x^2 + y^2\right)^{3/2}\,\eta b}$$

# Longitudinal and Transverse response GL and GT

For large distance, the asymptotic results from above readily give the real-space responses along and transverse to the connecting vector.
For small distances we need another calculation.

## GL

Large distances:

$$G_L\ (\rho) = \mathrm{Gxx}\ (x = \rho,\ y = 0) = \frac{1}{2\,\pi\,\eta_b\,\rho} \qquad (\rho >> \lambda)$$

Small distances:

First simplify the full expression as much as possible:

```
In[•]:= GxxA = Simplify[
          vxSurfaceN //. {ξ → 1, η → 1, Fx → 1, λ → Sqrt[ηb] * β, ω → I}, {q > 0, ηb > 0}];

In[•]:= GxxA = Simplify[GxxA //. {Sqrt[qx^2 + qy^2] → q, (qx^2 + qy^2) → q^2}, {q > 0, ηb > 0}];

In[•]:= GxxA = Simplify[GxxA /. {qy → Sqrt[q^2 - qx^2]}, {q > 0, x > 0}];

In[•]:= GxxB = GxxA //. {q → Q * a, qx → Qx * a}; (* a is an expansion parameter *)

In[•]:= % //. γ → 0;

In[•]:= % //. (1 + a^2 Q^2 β^2 ηb) -> (a^2 Q^2 β^2 ηb);

In[•]:= % //. (1 + a^2 Q^2) -> (a^2 Q^2);

In[•]:= FullSimplify[%, {Q > 0, a > 0, ηb > 0, β > 0}]
```

Out[•]=

$$\left(a\,Q\,\left(2\,Q^2-Qx^2\right)\,\eta b^{3/2}+4\,a^3\,Q^3\,\left(-Q^2+Qx^2\right)\,\eta b^{5/2}+4\,a^2\,Q^2\,(Q-Qx)\,(Q+Qx)\,\sqrt{\left(1+a^2\,Q^2\right)\,\eta b^5}+\left(-2\,Q^2+Qx^2\right)\,\eta b\,\sqrt{\eta b+a^2\,Q^2\,\eta b}\right)\Big/\left(2\,a\,Q^3\,\eta b\,\left(-a\,Q\,\eta b^{3/2}+2\,a^3\,Q^3\,\eta b^{5/2}-2\,a^2\,Q^2\,\sqrt{\left(1+a^2\,Q^2\right)\,\eta b^5}+\eta b\,\sqrt{\eta b+a^2\,Q^2\,\eta b}\right)\right)$$

Then expand in large q

```
In[•]:= Series[%, {a, Infinity, 1}]
```

Out[•]=

$$\frac{-Q^2+Qx^2}{Q^3\,\eta b\,a}+O\left[\frac{1}{a}\right]^2$$

After inverting to real space and setting (x = ρ, y = 0):

$$G_L\,(\rho)\;=\;\frac{1}{2\,\pi\,\eta_b\,\rho}\qquad(\rho << \lambda)$$

## ■ GT

Large distances

$$G_T\ (\rho)\ = Gxx\ (x = 0,\ y = \rho)\ = \frac{1}{4\,\pi\,\eta_b\,\rho} \qquad (\rho >> \lambda)$$

Small distances

Here the inversion to real space requires a more complicated analysis than for GL.

We extract the term proportional to qx^2.

In[ ]:=
```
CoefQx = Coefficient[GxxA, qx^2];
```

Extract the rest and invert it to real space.

In[ ]:=
```
FullSimplify[GxxA - CoefQx * qx^2]
```

Out[ ]=
$$-\frac{1}{q\,\eta b}$$

In[ ]:=
```
Integrate[q * % * Exp[I * q * ρ * Cos[p]],
  {p, 0, 2 Pi}, Assumptions → {q > 0, ρ > 0}] / (2 Pi)^2
```

Out[ ]=
$$-\frac{\text{BesselJ}[0,\ q\,\rho]}{2\,\pi\,\eta b}$$

In[ ]:=
$$\text{Integrate}\left[-\frac{\text{BesselJ}[0,\ q\,\rho]}{2\,\pi\,\eta b},\ \{q,\ 0,\ \text{Infinity}\},\ \text{Assumptions} \to \rho > 0\right]$$

Out[ ]=
$$-\frac{1}{2\,\pi\,\eta b\,\rho}$$

Go back to the more complicated qx^2 term and invert it to real space.

In[ ]:=
```
Integrate[q^3 * Cos[p]^2 * CoefQx * Exp[I * q * ρ * Sin[p]],
   {p, 0, 2 Pi}, Assumptions → {q > 0, ρ > 0}] / (2 Pi)^2;
```

In[ ]:=
```
FullSimplify[% * ρ / BesselJ[1, q ρ]];
```

In[ ]:= `% //. {γ → 0}`

Out[ ]= $$\left(8\,q^4\,\beta\,(-1+\eta b)\,\eta b^{3/2}-2\,\eta b\sqrt{\left(1+q^2\right)\left(1+q^2\,\beta^2\,\eta b\right)}+q^3\left(8\sqrt{1+q^2}\,\beta\,\eta b^{3/2}-8\,\beta\sqrt{\left(1+q^2\right)\eta b^5}-8\,(-1+\eta b)\,\eta b\sqrt{1+q^2\,\beta^2\,\eta b}\right)+2\,q^2\left(\beta\,\eta b^{3/2}+4\,(-1+\eta b)\,\eta b\sqrt{\left(1+q^2\right)\left(1+q^2\,\beta^2\,\eta b\right)}\right)\right)\Big/\left(4\,\pi\,q\,\eta b\left(4\,q^4\,\beta\,(-1+\eta b)\,\eta b^{3/2}-2\,\eta b\sqrt{\left(1+q^2\right)\left(1+q^2\,\beta^2\,\eta b\right)}+q^3\left(4\sqrt{1+q^2}\,\beta\,\eta b^{3/2}-4\,\beta\sqrt{\left(1+q^2\right)\eta b^5}-4\,(-1+\eta b)\,\eta b\sqrt{1+q^2\,\beta^2\,\eta b}\right)+2\,q^2\left(\beta\,\eta b^{3/2}+2\,(-1+\eta b)\,\eta b\sqrt{\left(1+q^2\right)\left(1+q^2\,\beta^2\,\eta b\right)}\right)\right)\right)$$

To extract the leading dependence on $\rho$, we change from q to k = q $\rho$

In[ ]:= `% //. {q → k / ρ};`

In[ ]:= `GT1 = FullSimplify[%, {k > 0, ρ > 0, β > 0}];`

Now expand in large distances, the numerator and denominator separately.

In[ ]:= `Series[Numerator[GT1], {ρ, 0, 5}];`

In[ ]:= `GT1Num = FullSimplify[Normal[%], {k > 0, ρ > 0, β > 0, ηb > 0}]`

Out[ ]= $$-\frac{\sqrt{\eta b}\,\left(3+\left(-2+\beta^2\right)\eta b\right)\rho^5}{2\,\beta}$$

In[ ]:= `Series[Denominator[GT1], {ρ, 0, 4}];`

In[ ]:= `GT1Den = FullSimplify[Normal[%], {k > 0, ρ > 0, β > 0, ηb > 0}]`

Out[ ]= $$-\frac{2\,k\,\pi\,\eta b^{3/2}\,\left(2+\left(-1+\beta^2\right)\eta b\right)\rho^4}{\beta}$$

In[ ]:= `FullSimplify[GT1Num / GT1Den, {k > 0, ρ > 0, β > 0, ηb > 0}]`

Out[ ]= $$\frac{\left(3+\left(-2+\beta^2\right)\eta b\right)\rho}{4\,k\,\pi\,\eta b\,\left(2+\left(-1+\beta^2\right)\eta b\right)}$$

Integrate over k and add up the two terms.

In[ ]:= Integrate[% * BesselJ[1, k], {k, 0, Infinity}] / ρ^2 - $\frac{1}{2\,\pi\,\rho\,\eta b}$

Out[ ]= $-\frac{1}{2\,\pi\,\eta b\,\rho}+\frac{3+\left(-2+\beta^2\right)\,\eta b}{4\,\pi\,\eta b\,\left(2+\left(-1+\beta^2\right)\,\eta b\right)\,\rho}$

In[ ]:= Together[%]

Out[ ]= $\frac{-1-\beta^2\,\eta b}{4\,\pi\,\eta b\,\left(2-\eta b+\beta^2\,\eta b\right)\,\rho}$

The final result:

$$G_T\ (\rho)\ =\ \frac{1}{4\,\pi\,\eta_b}\ \frac{\eta+\beta^2\,\eta b}{2\,\eta+\left(-1+\beta^2\right)\,\eta b}\ \frac{1}{\rho}\qquad (\rho << \lambda)$$

# Plot $G_L$

Numerical plot without asymptotes

In[ ]:= GLReal[r_, ηb_, β_, γ_] :=

$$\text{NIntegrate}\Big[\Big(\pi\,\Big(-\sqrt{1+\beta^2\,q^2\,\eta b}\,\Big(q\,\sqrt{1+q^2}\,\gamma+2\,q^4\,\gamma\,(-1+\eta b)-2\,q^3\,\left(\sqrt{1+q^2}\,\gamma-4\,\eta b\right)\,(-1+\eta b)+2\,\sqrt{1+q^2}\,\eta b-8\,q^2\,\sqrt{1+q^2}\,(-1+\eta b)\,\eta b\Big)+\beta\,q^2\,\Big(2\,q^3\,\gamma\,(-1+\eta b)\,\sqrt{\eta b}+2\,\eta b^{3/2}+q\,\sqrt{\eta b}\,\left(\gamma-8\,\sqrt{1+q^2}\,(-1+\eta b)\,\eta b\right)+2\,q^2\,\Big(-4\,\eta b^{3/2}+4\,\eta b^{5/2}+\gamma\,\Big(\sqrt{\left(1+q^2\right)\,\eta b}-\sqrt{\left(1+q^2\right)\,\eta b^3}\Big)\Big)\Big)\Big)\,\Big(2\,\text{BesselJ}[2,\,q\,r]-\text{Hypergeometric0F1Regularized}\Big[2,\,-\frac{1}{4}\,q^2\,r^2\Big]\Big)\Big)\Big/\Big(2\,\eta b\,\sqrt{1+\beta^2\,q^2\,\eta b}\,\Big(q\,\sqrt{1+q^2}\,\gamma+2\,\sqrt{1+q^2}\,\eta b+4\,q^3\,(-1+\eta b)\,\eta b-4\,q^2\,\sqrt{1+q^2}\,(-1+\eta b)\,\eta b\Big)-2\,\beta\,q^2\,\eta b^{3/2}\,\Big(2\,\eta b+4\,q^2\,(-1+\eta b)\,\eta b+q\,\Big(\gamma-4\,\sqrt{1+q^2}\,(-1+\eta b)\,\eta b\Big)\Big)\Big),\,\{q,\,0,\,\text{Infinity}\}\Big]\Big/\,((2*\text{Pi})\text{^}2)-\frac{1}{2\,\pi\,r\,\eta b}$$

Plot together with asymptote

In[ ]:=
```
GLRealTable =
  Table[{Exp[Lr], GLReal[Exp[Lr], 100., 1.1547, 0.]}, {Lr, Log[1], Log[100], 0.1}];
```

In[ ]:=
```
Show[ListLogLogPlot[Abs[GLRealTable], PlotRange → All],
 LogLogPlot[1/(2 π ηb x) /. {ηb → 100}, {x, 1, 100}], AxesLabel → {"ρ/ξ", "η · ξ · G_L"}]
```

Out[ ]=

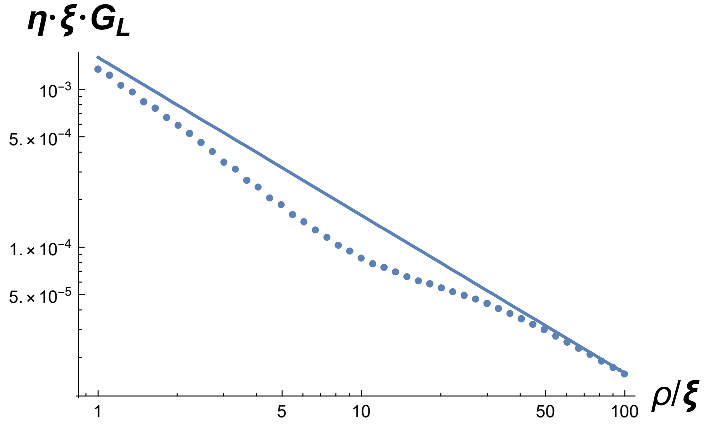


# Plot $G_T$

In[ ]:=
```
GTReal[r_, ηb_, β_, γ_] :=
 NIntegrate[(π (-Sqrt[1 + β^2 q^2 ηb] (q Sqrt[1 + q^2] γ + 2 q^4 γ (-1 + ηb) - 2 q^3
          (Sqrt[1 + q^2] γ - 4 ηb) (-1 + ηb) + 2 Sqrt[1 + q^2] ηb - 8 q^2 Sqrt[1 + q^2] (-1 + ηb) ηb) +
       β q^2 (2 q^3 γ (-1 + ηb) Sqrt[ηb] + 2 ηb^(3/2) + q Sqrt[ηb] (γ - 8 Sqrt[1 + q^2] (-1 + ηb) ηb) +
          2 q^2 (-4 ηb^(3/2) + 4 ηb^(5/2) + γ (Sqrt[(1 + q^2) ηb] - Sqrt[(1 + q^2) ηb^3])))))
      BesselJ[1, q r]) / (q r ηb (-Sqrt[1 + β^2 q^2 ηb] (q Sqrt[1 + q^2] γ + 2 Sqrt[1 + q^2] ηb +
          4 q^3 (-1 + ηb) ηb - 4 q^2 Sqrt[1 + q^2] (-1 + ηb) ηb) +
       β q^2 Sqrt[ηb] (2 ηb + 4 q^2 (-1 + ηb) ηb + q (γ - 4 Sqrt[1 + q^2] (-1 + ηb) ηb)))),
   {q, 0, Infinity}] / ((2 * Pi) ^2) - 1/(2 π r ηb)
```

```
In[ ]:= GTRealTable =
          Table[{Exp[Lr], GTReal[Exp[Lr], 100., 1.5, 1.]}, {Lr, Log[1], Log[100], 0.05}];
```

Plot together with asymptotes

```
In[ ]:= Show[ListLogLogPlot[Abs[GTRealTable], PlotRange → All],
         LogLogPlot[1/(4 π ηb x) /. {ηb → 100}, {x, 1, 100}],
         LogLogPlot[1/(4 π ηb x) * ((ηb * β^2 + 1)/((β^2 - 1) ηb + 2)) /. {ηb → 100, β → 1.5}, {x, 1, 100}],
         AxesLabel → {"ρ/ξ", "η · ξ · G_T"}]
```

Out[ ]=

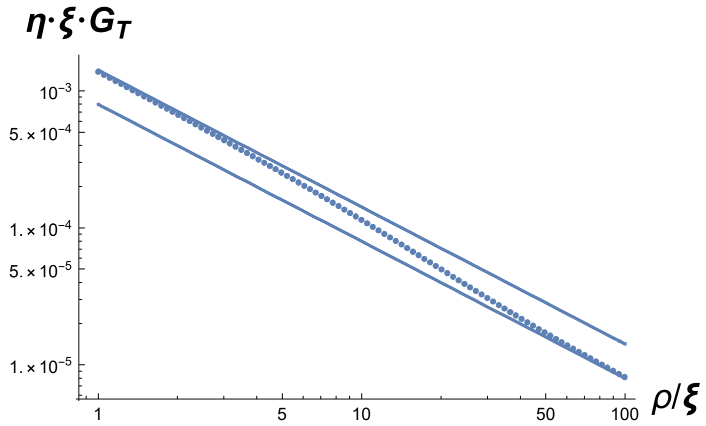


# Perpendicular response $G_P$ ($G_{zz}$)

To simplify the calculation we replace the 2D wavevector (qx,qy) by the scalar q (thanks to the xy symmetry).
We first rewrite all fields in this form.

```
In[ ]:= v2D[q_, z_] = v[qx, qy, z] //. {qy → 0, qx → q};

In[ ]:= u2D[q_, z_] = u[qx, qy, z] //. {qy → 0, qx → q};

In[ ]:= p2D[q_, z_] = p[qx, qy, z] //. {qy → 0, qx → q};

In[ ]:= {v2Dx[q_, z_], v2DNA[q_, z_], v2Dz[q_, z_]} = v2D[q, z];

In[ ]:= {u2Dx[q_, z_], u2DNA[q_, z_], u2Dz[q_, z_]} = u2D[q, z];

In[ ]:= σ2Dvxz = FullSimplify[η (D[v2Dx[q, z], z] + I q v2Dz[q, z]), q > 0];

In[ ]:= σ2Dvzz = FullSimplify[(2 η D[v2Dz[q, z], z] - p2D[q, z]), q > 0];

In[ ]:= σ2Duxz = FullSimplify[G (D[u2Dx[q, z], z] + I q u2Dz[q, z]) /. {G → (ηb - η) I ω}];

In[ ]:= σ2Duzz = Simplify[2 G D[u2Dz[q, z], z] + (K - 2 G / 3) (I q u2Dx[q, z] + D[u2Dz[q, z], z])];
```

Then, as above, solve for the boundary conditions, except that now the force is in the z direction.

```
In[ ]:= s5 = Solve[
    {σ2Dvxz + σ2Duxz == 0, σ2Dvzz + σ2Duzz == Fz - γ (q^2) u2Dz[q, z], I * ω * u2Dx[q, z] ==
      v2Dx[q, z], I * ω * u2Dz[q, z] == v2Dz[q, z]} /. z → 0, {C6, C4, D6, E2}];

In[ ]:= vz2DSurface = v2Dz[q, 0] /. s5[[1]];

In[ ]:= Gzz = Simplify[vz2DSurface, q > 0];
```

Small q (large $\rho$)

```
In[ ]:= GzzSmallq = Normal[Series[Gzz, {q, 0, 0}]]
```

Out[ ]= $-\frac{Fz}{2\, q\, \eta b} + \frac{i\, Fz\, \gamma}{4\, \eta b^2\, \omega}$

For inversion to real space we go back to 2D wavevector:

```
In[ ]:= InverseFourierTransform[1/(qx^2 + qy^2)^(1/2), {qx, qy}, {x, y}]
```

Out[ ]= $\frac{1}{\sqrt{x^2 + y^2}}$

$$G_P(\rho) = \frac{1}{4\,\pi\,\eta_b\,\rho} \qquad (\rho >> \max(\lambda, l_{ec}))$$

Large q (small $\rho$)

Simplify full expression as much as possible.

```
In[ ]:= GzzA = Simplify[
    vz2DSurface //. {ξ → 1, η → 1, Fz → 1, λ → Sqrt[ηb] * β, ω → I}, {q > 0, ηb > 0}];
```

Assume $\eta$b >> 1 (actually $\eta$b/$\eta$ >> 1)

```
In[ ]:= GzzB = Simplify[GzzA //. {ηb → x^2}, {q > 0, x > 0}]
```

Out[ ]= $-\left(\left(2\, q^2\, x^2 \left(q^2\, x\, \beta - \sqrt{(1 + q^2)\,(1 + q^2\, x^2\, \beta^2)}\right)\right)\right/$

$\left(-4\, q^5\, x^5\, (-1 + x^2)\, \beta + 2\, x^2 \sqrt{(q^2 + q^4)\,(1 + q^2\, x^2\, \beta^2)} - \right.$

$2\, q^3\, x^4 \left(x\, \beta + 2\,(-1 + x^2) \sqrt{(1 + q^2)\,(1 + q^2\, x^2\, \beta^2)}\right) + q^2 \sqrt{(1 + q^2)\,(1 + q^2\, x^2\, \beta^2)}\; \gamma +$

$q\,(-1 + x^2) \left(2\, x^2 \sqrt{(1 + q^2)\,(1 + q^2\, x^2\, \beta^2)} + \sqrt{(q^2 + q^4)\,(1 + q^2\, x^2\, \beta^2)}\; \gamma\right) -$

$$q^4\left(-4x^4\left(-1+x^2\right)\sqrt{1+q^2x^2\beta^2}+\beta\left(4\sqrt{1+q^2}\,x^5-4\sqrt{1+q^2}\,x^7+x^3\gamma\right)\right)\Bigg)\Bigg)+$$

$$\left(x^2\left(-q^2x\beta+\sqrt{\left(1+q^2\right)\left(1+q^2x^2\beta^2\right)}\right)\right)\Big/$$

$$\Bigg(4q^5x^5\left(-1+x^2\right)\beta-2x^2\sqrt{\left(q^2+q^4\right)\left(1+q^2x^2\beta^2\right)}+$$

$$2q^3x^4\left(x\beta+2\left(-1+x^2\right)\sqrt{\left(1+q^2\right)\left(1+q^2x^2\beta^2\right)}\right)-q^2\sqrt{\left(1+q^2\right)\left(1+q^2x^2\beta^2\right)}\,\gamma-$$

$$q\left(-1+x^2\right)\left(2x^2\sqrt{\left(1+q^2\right)\left(1+q^2x^2\beta^2\right)}+\sqrt{\left(q^2+q^4\right)\left(1+q^2x^2\beta^2\right)}\,\gamma\right)+$$

$$q^4\left(-4x^4\left(-1+x^2\right)\sqrt{1+q^2x^2\beta^2}+\beta\left(4\sqrt{1+q^2}\,x^5-4\sqrt{1+q^2}\,x^7+x^3\gamma\right)\right)\Bigg)+$$

$$\Bigg(2q\Bigg(-q^3x^5\beta+q^2x^2\left(-1+x^2\right)\sqrt{1+q^2x^2\beta^2}+q\left(-1+x^2\right)\sqrt{\left(1+q^2\right)\left(1+q^2x^2\beta^2\right)}+$$

$$\sqrt{\left(q^2+q^4\right)\left(1+q^2x^2\beta^2\right)}\Bigg)\Bigg)\Big/\Bigg(4q^5x^5\left(-1+x^2\right)\beta-2x^2\sqrt{\left(q^2+q^4\right)\left(1+q^2x^2\beta^2\right)}+$$

$$2q^3x^4\left(x\beta+2\left(-1+x^2\right)\sqrt{\left(1+q^2\right)\left(1+q^2x^2\beta^2\right)}\right)-q^2\sqrt{\left(1+q^2\right)\left(1+q^2x^2\beta^2\right)}\,\gamma-$$

$$q\left(-1+x^2\right)\left(2x^2\sqrt{\left(1+q^2\right)\left(1+q^2x^2\beta^2\right)}+\sqrt{\left(q^2+q^4\right)\left(1+q^2x^2\beta^2\right)}\,\gamma\right)+$$

$$q^4\left(-4x^4\left(-1+x^2\right)\sqrt{1+q^2x^2\beta^2}+\beta\left(4\sqrt{1+q^2}\,x^5-4\sqrt{1+q^2}\,x^7+x^3\gamma\right)\right)\Bigg)+$$

$$\left(2q^2\left(-1+x^2\right)\left(1+q^2x^2\beta^2-qx\beta\sqrt{1+q^2x^2\beta^2}\right)\right)\Big/$$

$$\Bigg(2\sqrt{1+q^2}\,x^2+4q^5x^4\left(-1+x^2\right)\beta^2-4q^4x^3\left(-1+x^2\right)\beta\left(\sqrt{1+q^2}\,x\beta+\sqrt{1+q^2x^2\beta^2}\right)+$$

$$2q^2x\Bigg(2\sqrt{1+q^2}\,x+\sqrt{1+q^2}\,x^3\left(-2+\beta^2\right)+2\beta\sqrt{\left(q^2+q^4\right)\left(1+q^2x^2\beta^2\right)}+$$

$$2x^4\beta\sqrt{\left(q^2+q^4\right)\left(1+q^2x^2\beta^2\right)}-x^2\beta\left(\sqrt{1+q^2x^2\beta^2}+4\sqrt{\left(q^2+q^4\right)\left(1+q^2x^2\beta^2\right)}\right)\Bigg)+$$

$$q\sqrt{1+q^2}\,\gamma+q^3x\Bigg(4x^3+4x^2\beta\sqrt{\left(1+q^2\right)\left(1+q^2x^2\beta^2\right)}+x\left(-4+\sqrt{1+q^2}\,\beta^2\gamma\right)-$$

$$\beta\left(4\sqrt{\left(1+q^2\right)\left(1+q^2 x^2 \beta^2\right)}+\sqrt{1+q^2 x^2 \beta^2}\ \gamma\right)\Bigg)\Bigg)$$

```
In[•]:= FullSimplify[GzzB //. {(1 + β^2 q^2 x^2) → β^2 q^2 x^2}, {x > 0, q > 0, β > 0}]
```

Out[•]= $-\frac{1}{2\,q\,x^2+q^2\,\gamma}$

Invert to real space as before

```
In[•]:= Integrate[Exp[I * q * ρ * Cos[ϕ]] / (q (q + κ)), {ϕ, 0, 2 * Pi}, Assumptions → q ρ ∈ ℝ]
```

Out[•]= $\frac{2\,\pi\,\text{BesselJ}[0,\,q\,\rho]}{q\,(q+\kappa)}$

```
In[•]:= FullSimplify[q (2 π BesselJ[0, q ρ])/(q (q + κ)) //. q → k / ρ]
```

Out[•]= $\frac{2\,\pi\,\rho\,\text{BesselJ}[0,\,k]}{k+\kappa\,\rho}$

```
In[•]:= Integrate[%, {k, 0, Infinity}, Assumptions → {ρ κ ∈ ℝ, ρ κ ≥ 0}] / (ρ * (2 Pi) ^2)
```

Out[•]= $\frac{1}{4\,\pi}\left(2\,\text{BesselJ}[0,\,\kappa\,\rho]\,\text{Log}\left[\frac{2}{\kappa\,\rho}\right]+\pi\,\text{StruveH}[0,\,\kappa\,\rho]-2\,\text{Hypergeometric0F1Regularized}^{(1,0)}\left[1,\,-\frac{1}{4}\,\kappa^2\,\rho^2\right]\right)$

```
In[•]:= Series[1/(2 π) (BesselJ[0, x] Log[2/x] + 1/2 π StruveH[0, x] -
            Hypergeometric0F1Regularized^(1,0)[1, -1/4 x^2]), {x, 0, 0}]
```

Out[•]= $\frac{\text{Log}\left[\frac{2}{x}\right]-\text{Hypergeometric0F1Regularized}^{(1,0)}[1,\,0]}{2\,\pi}+O[x]^1$

```
In[•]:= N[-Hypergeometric0F1Regularized^(1,0)[1, 0] + EulerGamma]
```

Out[•]= 0.

```
In[•]:= Gp = ((Log[2/x] - EulerGamma)/(2 π γ)) //. x → ρ κ
```

Out[•]= $\frac{-\text{EulerGamma}+\text{Log}\left[\frac{2}{\kappa\,\rho}\right]}{2\,\pi\,\gamma}$

We now rewrite this result in terms of the original parameters.

In[ ]:= **Gp = % //. $\kappa \to \frac{2\,\eta b}{\gamma}$**

Out[ ]= $\frac{-\text{EulerGamma} + \text{Log}\left[\frac{\gamma}{\eta b\,\rho}\right]}{2\,\pi\,\gamma}$

$\gamma$ is really the actual $\gamma$ divided by i$\omega$. We also introduce the elasto-capillary length:

$$\text{lec} = \frac{\gamma\text{real}}{\text{I}\,\omega\,\eta\text{b}}$$

$$\frac{\gamma}{\text{r}\,\eta\text{b}} = \frac{\gamma\text{real}}{\text{I}\,\omega\,\eta\text{b}\,\text{r}} = \frac{\text{lec}}{\text{r}}$$

$$\frac{1}{\gamma} = \frac{\text{I}\,\omega}{\gamma\text{real}} = \frac{\text{I}\,\omega}{\text{lec}\,\text{I}\,\omega\,\eta\text{b}} = \frac{1}{\text{lec}\;\eta\text{b}}$$

So, the final result :

$$\mathbf{G_P\ (\rho) = \frac{-\text{EulerGamma} + \text{Log}\left[\frac{\text{lec}}{\rho}\right]}{2\,\pi\,\text{lec}\;\eta_b}} \qquad (\rho << \min\ (\lambda,\ l_{ec}))$$

Intermediate regime

We find graphically that GP goes like 1/q in this regime (see plot below). So, we are after the coefficient.

As above, we expand in large $\eta$b, the numerator and denominator separately:

In[ ]:= **GzzB = Simplify[GzzA //. {ηb → x^2}, {q > 0, x > 0}]**

In[ ]:= **GzzB = FullSimplify[GzzB /. {q → 1}, {x > 0, q > 0, β > 0}]**

In[ ]:= **FullSimplify[Series[Numerator[GzzB], {x, Infinity, 0}], {x > 0, β > 0}]**

Out[ ]= $\left(6 - 4\sqrt{2}\right)\beta\left(-1 + \beta^2\right)x^5 + \frac{\left(-7 + 4\sqrt{2} + \left(26 - 16\sqrt{2}\right)\beta^2 + \left(6 - 4\sqrt{2}\right)\beta^4\gamma\right)x^3}{2\beta} + \frac{\left(3 - 2\sqrt{2} + \left(19 - 8\sqrt{2}\right)\beta^2 + 2\left(7 - 4\sqrt{2}\right)\beta^4\gamma\right)x}{4\beta^3} + O\left[\frac{1}{x}\right]^1$

In[ ]:= FullSimplify[Series[Denominator[GzzB], {x, Infinity, 0}], {x > 0, β > 0}]

Out[ ]=
$$\frac{4\left(-3+2\sqrt{2}\right)\left(-1+\beta^2\right)^2 x^7}{\beta}+\frac{2\left(-1+\beta^2\right)\left(-19+12\sqrt{2}+\left(-6+4\sqrt{2}\right)\beta^2\gamma\right)x^5}{\beta}+$$
$$\frac{1}{4\beta^5}\left(3-2\sqrt{2}+4\left(-3+2\sqrt{2}\right)\beta^2+8\left(-13+8\sqrt{2}\right)\beta^6\gamma+\right.$$
$$\left.4\left(-3+2\sqrt{2}\right)\beta^8\gamma^2+2\beta^4\left(-57+32\sqrt{2}+\left(14-8\sqrt{2}\right)\gamma\right)\right)x^3+$$
$$\frac{1}{8\beta^7}\left(-6+4\sqrt{2}-\beta^2+4\left(-19+8\sqrt{2}\right)\beta^6\gamma+4\left(-7+4\sqrt{2}\right)\beta^8\gamma^2+\right.$$
$$\left.2\beta^4\left(13-8\sqrt{2}+\left(-6+4\sqrt{2}\right)\gamma\right)\right)x+O\left[\frac{1}{x}\right]^1$$

Take the leading term in each.

In[ ]:= FullSimplify$\left[\left(6-4\sqrt{2}\right)\beta\left(-1+\beta^2\right)x^5 \Big/ \frac{4\left(-3+2\sqrt{2}\right)\left(-1+\beta^2\right)^2 x^7}{\beta}\right]$

Out[ ]=
$$-\frac{\beta^2}{2x^2\left(-1+\beta^2\right)}$$

The final result (after inverting to real space):

$$G_P\ (\rho)=\frac{1}{4\pi\eta_b\rho}\frac{\beta^2}{\left(\beta^2-1\right)}\qquad (l_{ec} << \rho << \lambda)$$

# Plot $G_P$

## ■ Focus on large and intermediate distances

The full expression using numerical integration

In[ ]:= GzzRealNum[r_, ηb_, b_, γ_] :=

$$\text{NIntegrate}\left[-\frac{1}{r}k\left(\left(r^3\eta b\left(b k^2\sqrt{\eta b}-\sqrt{\left(k^2+r^2\right)\left(r^2+b^2k^2\eta b\right)}\right)\right)\Big/\right.\right.$$
$$\left(4k^4(-1+\eta b)\eta b^2\sqrt{r^2+b^2k^2\eta b}+k^2 r\gamma\sqrt{\left(k^2+r^2\right)\left(r^2+b^2k^2\eta b\right)}-\right.$$
$$4k^3(-1+\eta b)\eta b^2\sqrt{\left(k^2+r^2\right)\left(r^2+b^2k^2\eta b\right)}+2r^2\eta b\sqrt{k^2\left(k^2+r^2\right)\left(r^2+b^2k^2\eta b\right)}-$$

$$b\,k^3\,\eta b^{3/2}\left(k\,r\,\gamma + 2\,r^2\,\eta b + 4\,k^2\,(-1+\eta b)\,\eta b - 4\,k\,\sqrt{k^2+r^2}\,(-1+\eta b)\,\eta b\right) +$$

$$k\,r\,(-1+\eta b)\left(2\,r\,\eta b\sqrt{(k^2+r^2)\,(r^2+b^2\,k^2\,\eta b)} + \gamma\sqrt{k^2\,(k^2+r^2)\,(r^2+b^2\,k^2\,\eta b)}\right)\Bigg) -$$

$$\left(2\,b\,k^4\,r\,\eta b^{3/2} - 2\,k^2\,r\,\eta b\sqrt{(k^2+r^2)\,(r^2+b^2\,k^2\,\eta b)}\right)\Big/$$

$$\Bigg(4\,k^4\,(-1+\eta b)\,\eta b^2\sqrt{r^2+b^2\,k^2\,\eta b} + k^2\,r\,\gamma\sqrt{(k^2+r^2)\,(r^2+b^2\,k^2\,\eta b)} -$$

$$4\,k^3\,(-1+\eta b)\,\eta b^2\sqrt{(k^2+r^2)\,(r^2+b^2\,k^2\,\eta b)} + 2\,r^2\,\eta b\sqrt{k^2\,(k^2+r^2)\,(r^2+b^2\,k^2\,\eta b)} -$$

$$b\,k^3\,\eta b^{3/2}\left(k\,r\,\gamma + 2\,r^2\,\eta b + 4\,k^2\,(-1+\eta b)\,\eta b - 4\,k\,\sqrt{k^2+r^2}\,(-1+\eta b)\,\eta b\right) +$$

$$k\,r\,(-1+\eta b)\left(2\,r\,\eta b\sqrt{(k^2+r^2)\,(r^2+b^2\,k^2\,\eta b)} + \gamma\sqrt{k^2\,(k^2+r^2)\,(r^2+b^2\,k^2\,\eta b)}\right)\Bigg) +$$

$$\Bigg(2\,k\,r\,\Bigg(b\,k^3\,\eta b^{5/2} - k^2\,(-1+\eta b)\,\eta b\sqrt{r^2+b^2\,k^2\,\eta b} - k\,(-1+\eta b)$$

$$\sqrt{(k^2+r^2)\,(r^2+b^2\,k^2\,\eta b)} - \sqrt{k^2\,(k^2+r^2)\,(r^2+b^2\,k^2\,\eta b)}\Bigg)\Bigg)\Big/$$

$$\Bigg(4\,k^4\,(-1+\eta b)\,\eta b^2\sqrt{r^2+b^2\,k^2\,\eta b} + k^2\,r\,\gamma\sqrt{(k^2+r^2)\,(r^2+b^2\,k^2\,\eta b)} -$$

$$4\,k^3\,(-1+\eta b)\,\eta b^2\sqrt{(k^2+r^2)\,(r^2+b^2\,k^2\,\eta b)} + 2\,r^2\,\eta b\sqrt{k^2\,(k^2+r^2)\,(r^2+b^2\,k^2\,\eta b)} -$$

$$b\,k^3\,\eta b^{3/2}\left(k\,r\,\gamma + 2\,r^2\,\eta b + 4\,k^2\,(-1+\eta b)\,\eta b - 4\,k\,\sqrt{k^2+r^2}\,(-1+\eta b)\,\eta b\right) +$$

$$k\,r\,(-1+\eta b)\left(2\,r\,\eta b\sqrt{(k^2+r^2)\,(r^2+b^2\,k^2\,\eta b)} + \gamma\sqrt{k^2\,(k^2+r^2)\,(r^2+b^2\,k^2\,\eta b)}\right)\Bigg) +$$

$$\left(2\,k^2\,r\,(-1+\eta b)\left(r^2 + b\,k\left(b\,k\,\eta b - \sqrt{\eta b\,(r^2+b^2\,k^2\,\eta b)}\right)\right)\right)\Big/$$

$$\Bigg(k\,r^3\,\sqrt{k^2+r^2}\,\gamma + 2\,r^4\,\sqrt{k^2+r^2}\,\eta b + 4\,b^2\,k^5\,(-1+\eta b)\,\eta b^2 -$$

$$4\,b\,k^4\,(-1+\eta b)\,\eta b^{3/2}\left(b\sqrt{(k^2+r^2)\,\eta b} + \sqrt{r^2+b^2\,k^2\,\eta b}\right) +$$

```
k^3 (4 r^2 (-1 + ηb) ηb + b r γ (b Sqrt[k^2 + r^2] ηb - Sqrt[ηb (r^2 + b^2 k^2 ηb)]) -
    4 b (-ηb^(3/2) Sqrt[(k^2 + r^2) (r^2 + b^2 k^2 ηb)] + Sqrt[(k^2 + r^2) ηb (r^2 + b^2 k^2 ηb)])) +
  2 k^2 (r^2 ηb (2 Sqrt[k^2 + r^2] + (-2 + b^2) Sqrt[k^2 + r^2] ηb - b Sqrt[ηb (r^2 + b^2 k^2 ηb)]) +
    2 b (-2 ηb^(3/2) Sqrt[k^2 (k^2 + r^2) (r^2 + b^2 k^2 ηb)] + ηb^(5/2)
        Sqrt[k^2 (k^2 + r^2) (r^2 + b^2 k^2 ηb)] + Sqrt[k^2 (k^2 + r^2) ηb (r^2 + b^2 k^2 ηb)])))) *
  BesselJ[0, k], {k, 0, Infinity}] / (r * (2 * Pi))
```

In[ ]:=
```
GzzRealTable =
  Table[{Exp[Lr], GzzRealNum[Exp[Lr], 100., 1.5, 0.]}, {Lr, Log[1], Log[1000], 0.2}];
```

Plot the full expression together with the two asymptotes found above.

In[ ]:=
```
Show[ListLogLogPlot[Abs[GzzRealTable], PlotRange → All],
 LogLogPlot[(1/(4 π ηb x)) /. {ηb → 100}, {x, 1, 1000}],
 LogLogPlot[((β^2 / (β^2 - 1))/(4 π ηb x)) /. {ηb → 100, β → 1.5}, {x, 1, 1000}],
 AxesLabel → {"ρ/ξ", "η·ξ·G_P"}]
```

Out[ ]=

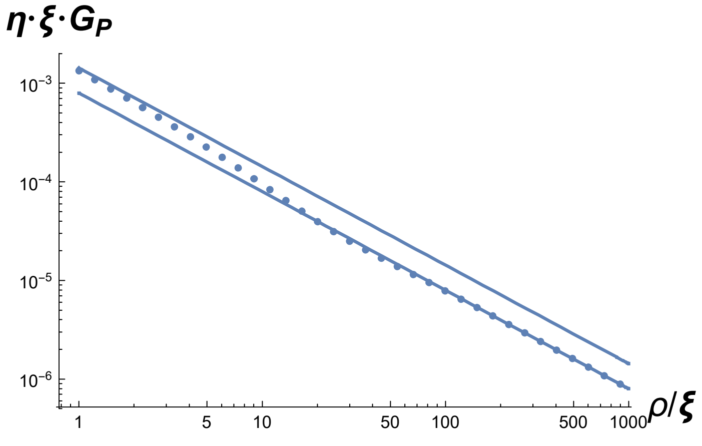


## Focus on short distances

Plot the full expression together with the two relevant asymptotes (short and intermediate distances).

In[ ]:=
```
GzzRealTable = Table[
  {Exp[Lr], GzzRealNum[Exp[Lr], 100., 1.5, 10000.]}, {Lr, Log[1], Log[1000], 0.2}];
```

In[ ]:=
```
Show[ListLogLogPlot[Abs[GzzRealTable], PlotRange → All],
 LogLogPlot[(1/(4 π ηb x)) /. {ηb → 100}, {x, 1, 1000}],
 LogLogPlot[((Log[2 / (2 ηb x / γ)] - EulerGamma)/(2 Pi γ)) /. {ηb → 100, γ → 10000}, {x, 1, 1000}],
 AxesLabel → {"ρ/ξ", "η·ξ·G_P"}]
```

Out[ ]=

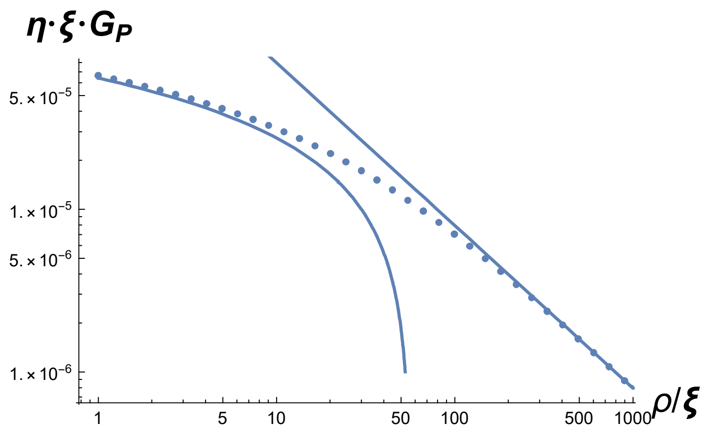

Supplement: Supplementary file 1 [file supplemental_detailed_calculation.pdf]
